# Supplementary material for: Influence of planets on debris disks in star clusters I: the 50 AU Jupiter
Source: arXiv:2306.01283 source file (2023-06-02)
Supplement: Supplementary file 1 [file appendix.tex]

\section{Extra figures about escaper properties}

\begin{figure}
    \begin{tabular}{c}
        \includegraphics[width=\columnwidth]{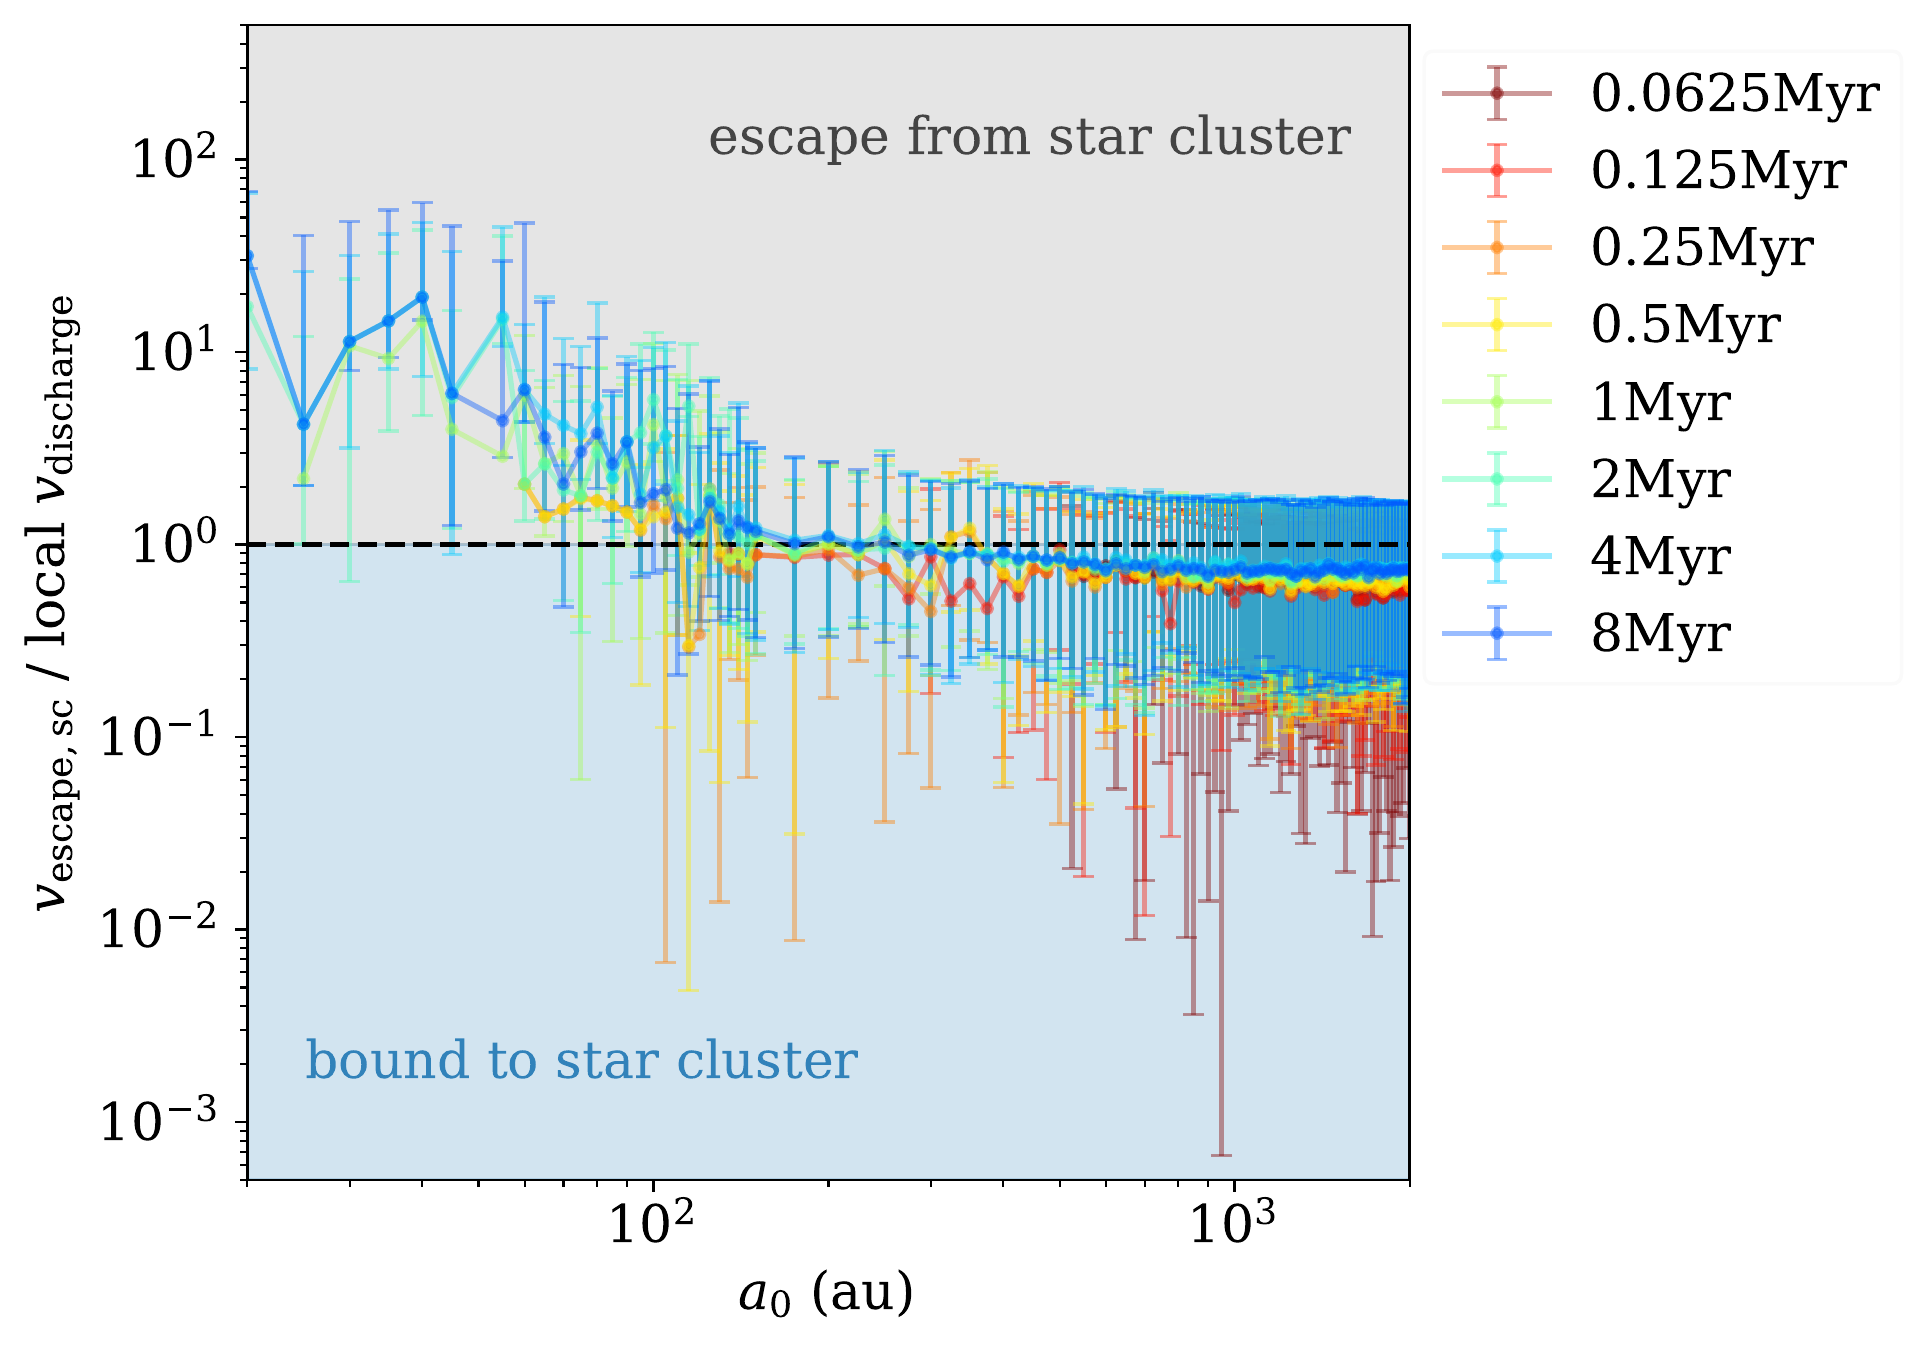} \\
        \includegraphics[width=\columnwidth]{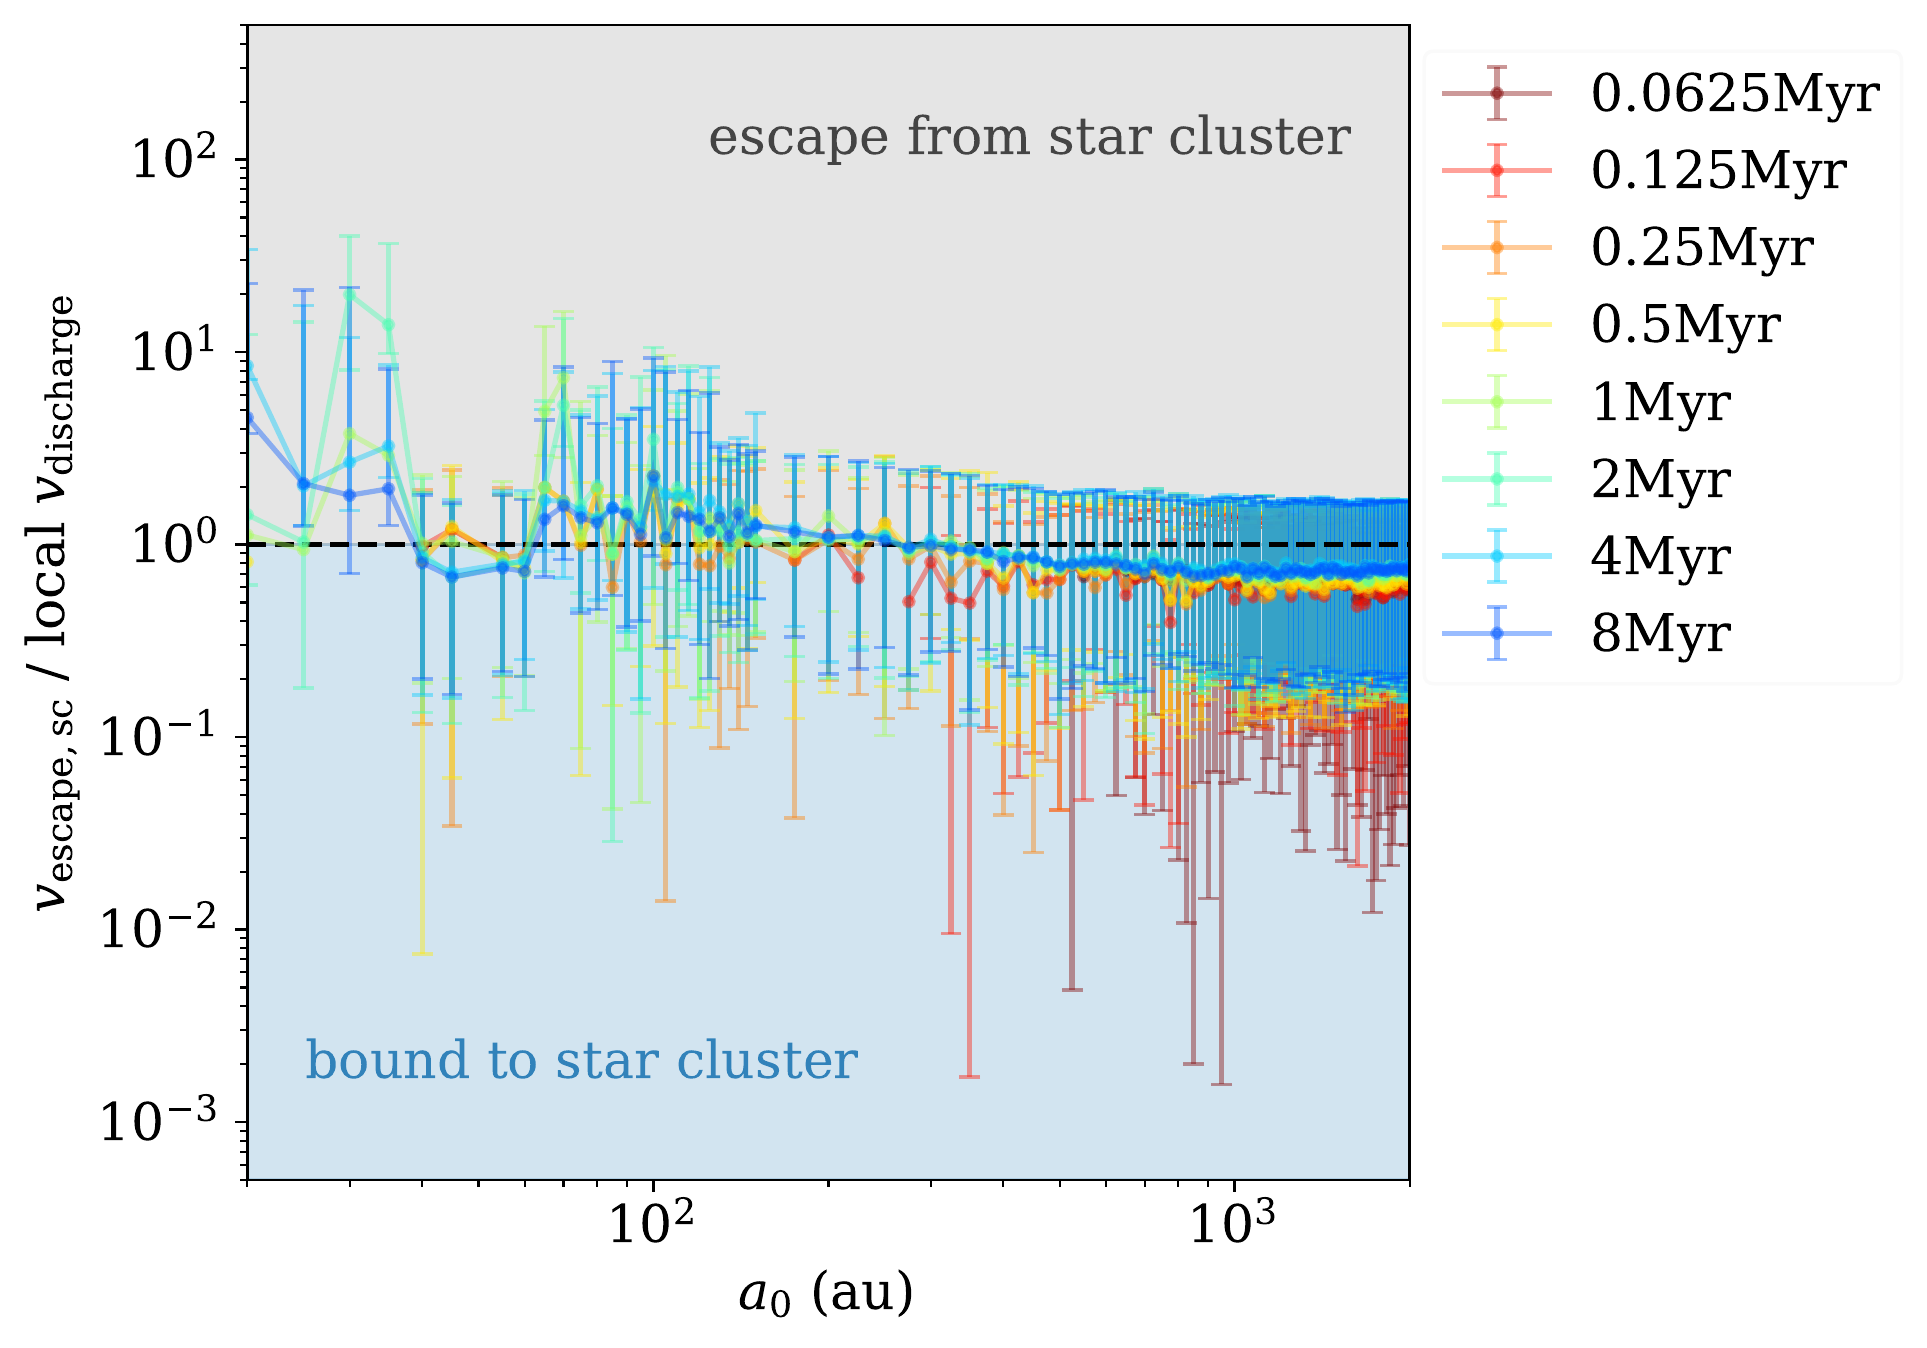} \\
    \end{tabular}
    \caption{Statistics of escape speed divided by the local discharge barrier speed of the star cluster ($v_\mathrm{escape,sc}~/~\mathrm{local}~v_\mathrm{discharge}$) of escapers which escape before 8~Myr, \ensemble{}. \emph{Top}: simulations without planet. \emph{Bottom}: simulations with \fifju{}. The solid point is the median of the data, while the error bar represents the range between the first quartile (25\%) to the third quartile (75\%) of the data. We identify the data representing particles escaping from the star cluster and bound to the star cluster with gray and blue filling colors, respectively.}
    \label{fig.8k_0_escapers_speed_over_a0early}
\end{figure}

\begin{figure}
    \begin{tabular}{c}
        \includegraphics[width=\columnwidth]{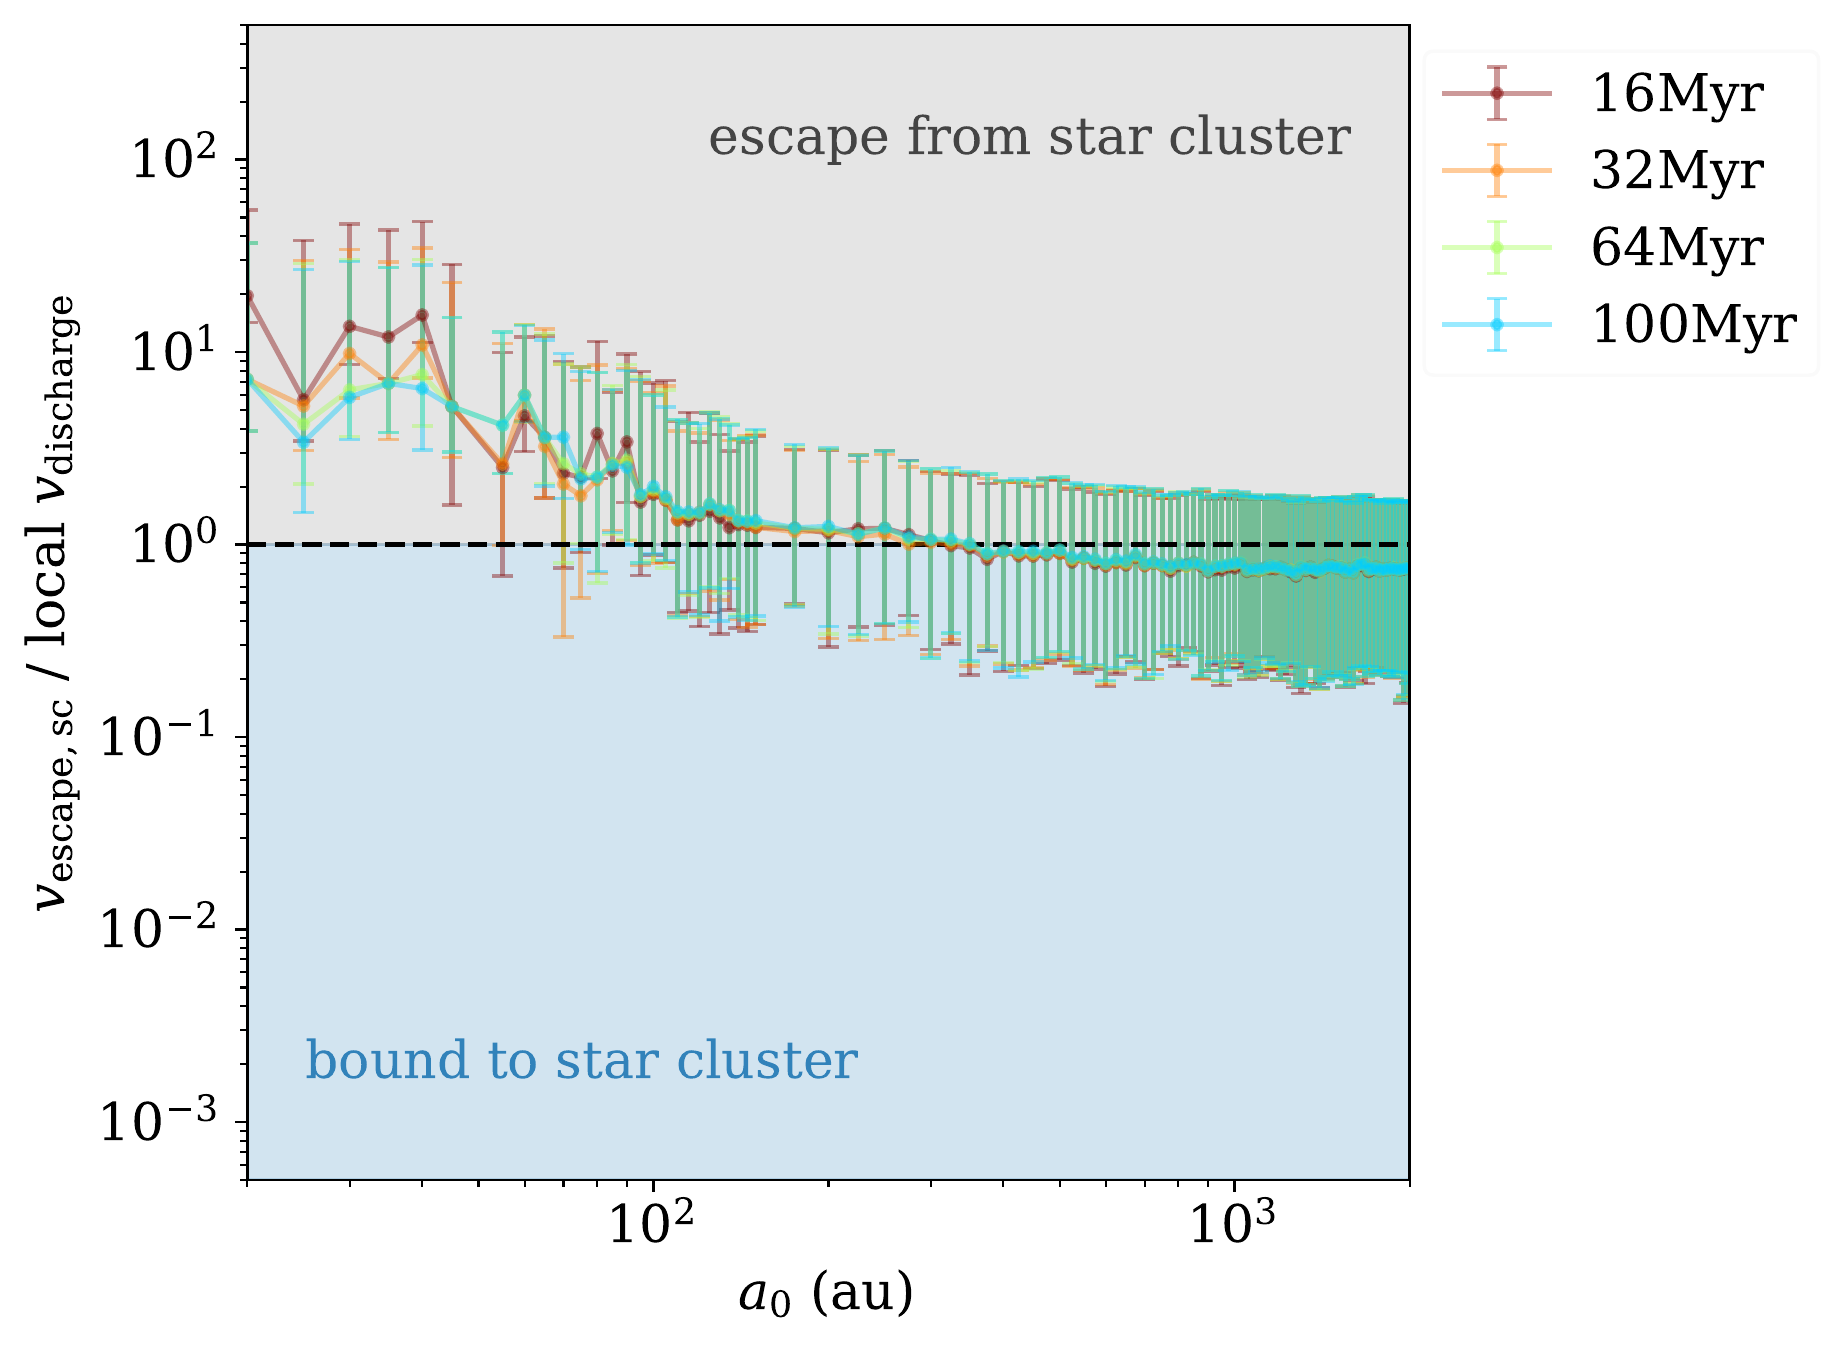} \\
        \includegraphics[width=\columnwidth]{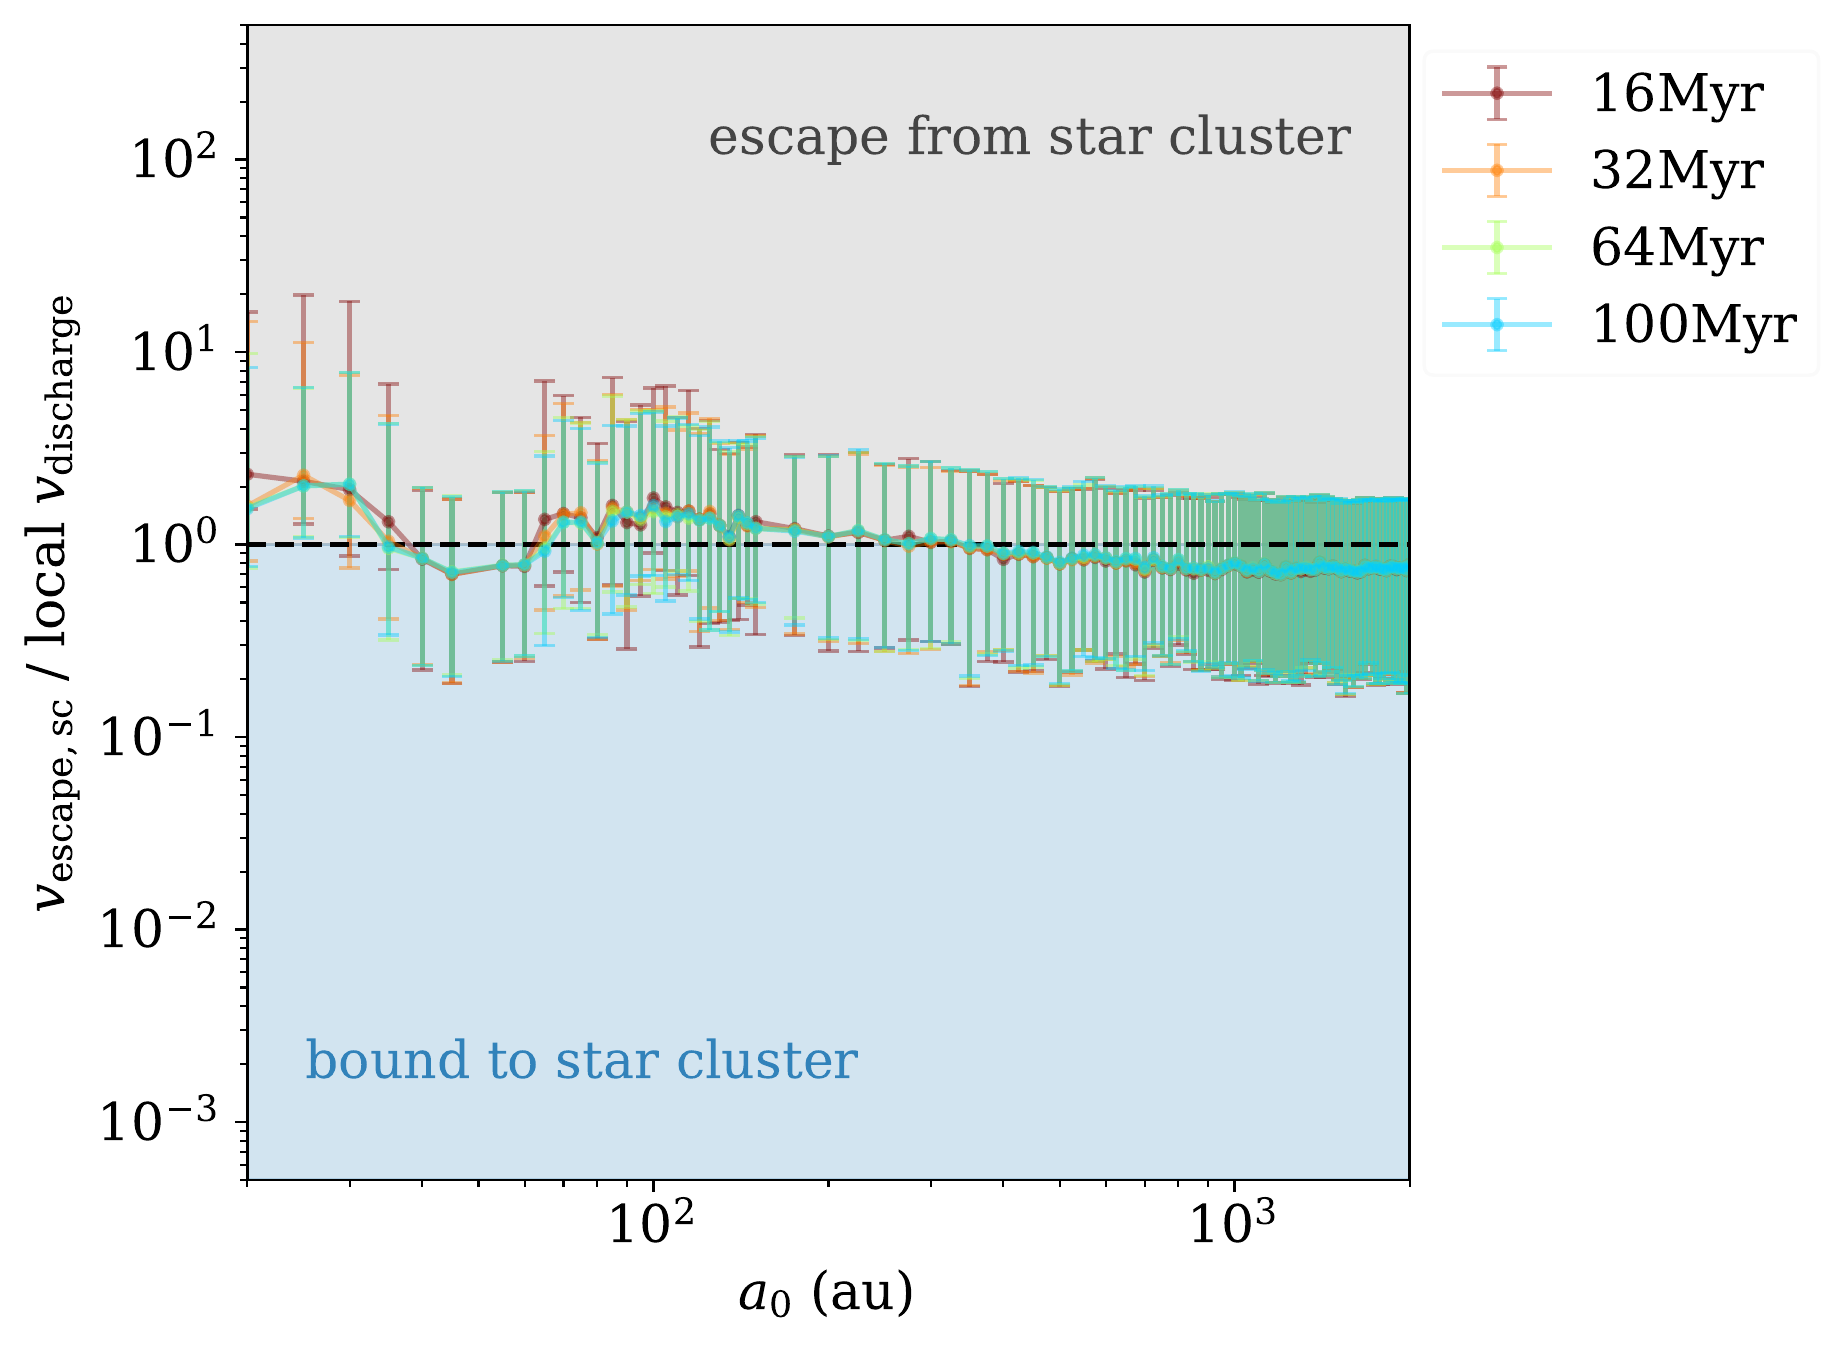} \\
    \end{tabular}
    \caption{Same as Figure~\ref{fig.8k_0_escapers_speed_over_a0early}, but only include escapers that escape after 16~Myr.}
    \label{fig.8k_0_escapers_speed_over_a0late}
\end{figure}
